# Supplementary material for: NeRF-Pose: A First-Reconstruct-Then-Regress Approach for Weakly-supervised 6D Object Pose Estimation
Source: arXiv:2203.04802 source file (2023-09-09)
Supplement: Supplementary file 1 [file 14_appendix.tex]

\newpage

\newpage

\section{Appendix}

The supplementary materials provide additional details and clarifications of the proposed approach. 
We start by discussing the utilized datasets. 
Then, in Sec.~\ref{sec:shape}, we analyse shape reconstruction quality of OBJ-NeRF.
And, in sec.~\ref{sec:network}, we describe the network architecture.
Sec.~\ref{sec:ransac} provides the pseudocode of our NeRF-enabled PnP+RANSAC algorithm used for pose estimation. Finally, in Sec.~\ref{sec:results}, the predicted poses are visualized.

\section{Dataset}
\label{sec:data}

LineMod (LM)~\cite{brachmann2014learning} and LineMod Occlusion (LMO)~\cite{brachmann2018learning} datasets are released under 
\hyperlink{https://creativecommons.org/licenses/by/4.0/}{Creative Commons Attribution 4.0 International License}. LM dataset consists of 15 texture-less household objects with discriminative color, shape, and size. Each sequence contains exactly one object with annotated poses. LMO dataset was built atop of the LM dataset by adding pose labels to all visible LM object to one on LM sequences. This introduced challenging test case with various levels of occlusion. However, the relative camera pose labels, needed for our weakly-supervised setting, are not provided in LM dataset. Moreover, images for on object do not come from the same video sequence with static scene. It means SfM and SLAM can not be performed on the scenes to estimate relative camera transformations. 
Thus, we derive relative camera pose labels from known object poses in different frames. This is only done for compute relative camera poses, and ground truth object poses are not used in the rest of the pipeline. 

\begin{figure}
   \centering
    \includegraphics[width=8cm]{figure/ext-hbd.png}
        \caption{The samples of our HBD-REXT dataset.  
        }
    \label{fig:exthbd}
\end{figure}

HomebrewedDB (HBD)~\cite{kaskman2019homebreweddb} dataset is released under
\hyperlink{http://campar.in.tum.de/personal/ilic/homebreweddb/files/LICENSE.html}{Creative Common Zero License}. It consists of 33 objects in 13 different scenes. And, 16 objects in 3 testing scenes are selected in BOP challenge test set. However, the real training images with 2D segmentation and camera relative pose labels are missing which are needed for our weakly-supervised approach. 
Based on the homebrewedDB toolkit in ~\cite{kaskman2019homebreweddb}, we extend the homebrewedDB dataset by capturing more real image sequences. 
To be more specific, we collect separated real training images for 16 objects used in the BOP challenge. As shown in Fig.~\ref{fig:exthbd}, the object model is on the markerboard, and the RGBD sequences of the objects are captured using Azure Kinect camera.
Only 2D object segmentation and relative camera poses are provided in our extension sequences. 

\section{Shape Analysis} \label{sec:shape}

Our main contribution is the object reconstructed as an implicit neural network in terms of OBJ-NeRF from weak labels. In this section, we analyze the quality of shape reconstruction reported in terms of the Chamfer distance, following~\cite{gkioxari2019mesh}. The Chamfer distance between two point clouds $P$ and $Q$ is given by

\begin{align}
\small
\mathcal{L}_{cham}(P, Q)= & \frac{1}{2|P|} \sum_{p \in P} \min_{q \in Q} \parallel p - q\parallel_2 \\
 & + \frac{1}{2|Q|}\sum_{q \in Q} \min_{p \in P}\parallel p - q\parallel_2.
\end{align}

\begin{table}
    \begin{center}
    \small
    \caption{Chamfer distance (millimeter) on LM and HBD objects. The numbers are the Chamfer distance between our reconstructed object model and the CAD model. 
    % And, Cubified denotes the Chamfer distance between the cubified mesh (defined in Sec.~\ref{sec:shape}) and CAD model.
    }
    \resizebox{0.48\textwidth}{!}{
    \begin{tabular}{c | c | c | c | c  | c | c | c  | c }
\toprule
\multirow{4}{*}{LM} 
 & obj01  & obj02 & obj04  & obj05   &  obj06 & obj08 & obj09 & obj10 \\
 & 2.36   & 3.07  & 2.43   & 2.56    &  2.40  & 2.24  & 2.52  & 3.96  \\
 \cline{1-9}
 & obj11  & obj12 & obj13  & obj14   &  obj15 & 	    &       &       \\
 & 2.15   & 3.11  & 3.46   & 3.47    &  2.44  &       &       &       \\
 \hline
\multirow{4}{*}{HBD}  & obj01  & obj03 & obj04  & obj08   &  obj09 & obj10 & obj12 & obj15 \\
 & 2.79   & 2.45  & 3.28   & 2.73    &  5.15  & 10.65 & 3.22  & 2.99  \\
\cline{1-9}
 & obj17  & obj18 & obj19  & obj22   &  obj23 & obj29 & obj32 & obj33 \\
 & 2.45   & 2.76  & 1.97   & 2.86    &  3.98  & 2.13  & 3.46  & 2.45  \\
\toprule
\end{tabular} }
\label{tab:shapeerror}
\end{center}
\end{table}

\begin{figure}
    \centering
    \includegraphics[width=8.5cm]{figure/lm-nerf.png}
        \caption{Qualitative results on OBJ-NeRF object reconstruction in LM and LM-O. LM and LM-O share the same training data in our settings. Columns (a) and (d) show the real object images which masks its background using 2D segmentation mask. Columns (b) and (e) are rendered from our well-trained object model. Columns (c) and (f) are the rendered NOCS-maps.}
    \label{fig:obj-nerf-lm}
\end{figure}

More precisely, we first uniformly sample 50K points both from ground truth and reconstructed polygon meshes as two point sets $P$ and $Q$. Then, the Chamfer distance is evaluated for the two produced point clouds. 
We convert our learned implicit object neural representation to the polygon mesh, by the following steps:
first, we uniformly sample $N \times N \times N$ grids inside the NeRF boundary box (shown in Fig.~\ref{fig:obj-nerf-m}), and predict the occupancy data for each voxel from OBJ-NeRF. Then, based on the volumetric data, we can build the polygon mesh using marching cubes algorithm~\cite{1987Marching}.

\begin{figure}
    \centering
    \includegraphics[width=8.5cm]{figure/hbd-nerf.png}
        \caption{Qualitative results on OBJ-NeRF object reconstruction in HBD.Columns (a) and (d) show the real object images which masks its background using 2D segmentation mask. Columns (b) and (e) are rendered from our well-trained object model. Columns (c) and (f) are the rendered NOCS-maps.}
    \label{fig:obj-nerf-hbd}
\end{figure}

% The numeric evaluation results are provided in Table~\ref{tab:shapeerror} where we make compare a shape error with a voxelization representation with the resolution $N=256$. We compare against cubified mesh~\cite{gkioxari2019mesh} in the same sampling resolutions. To obtain the cubified mesh in resolution $N$, the CAD model is first generated in a $N \times N \times N$ occupancy grid with respect to the object center. Then the meshes are regenerated in these grid cells. The voxelization algorithm is the one used in~\cite{Peng2020ECCV}.

The Fig.~\ref{fig:obj-nerf-lm} and Fig.~\ref{fig:obj-nerf-hbd} are the visualization results of our reconstructed implicit neural object compared to the real training images. Our weakly-supervised OBJ-NeRF reconstructs the objects precisely, both in object shape and color. As shown from the rendered NOCS-map in Fig.~\ref{fig:obj-nerf-lm}, the accurate object surface are reconstructed which provides the highly consistent labels for the training of pose regression network. 
Object 10 (brown industry object) in HBD dataset has the larger Chamfer distance (10.60) compared to other objects. As seen from Fig.~\ref{fig:obj-nerf-hbd}, the inside of the object can not be well reconstructed due to the symmetric property. And, moreover, some shape details are missing, e.g. the cat eyes and phone keyboards in Fig.~\ref{fig:obj-nerf-lm}. We also observe some white borderlines in Fig.\ref{fig:obj-nerf-hbd}. These minor shape errors are mainly from the imprecise 2D segmentation and pose labels. 

\section{Network Details}\label{sec:network}

Our approach, \textbf{NeRF-Pose}, includes two stages: \textit{multi-view neural object reconstruction} and \textit{single-view object pose estimation}. 
In the first stage, we reconstruct the object as OBJ-NeRF network from weak labels.
Then, in the second stage, we train a pose regression network supervised with NOCS-map labels rendered with the OBJ-NeRF.

\begin{figure}
    \setlength{\belowcaptionskip}{-1cm}
    \centering
    \includegraphics[width=8.5cm]{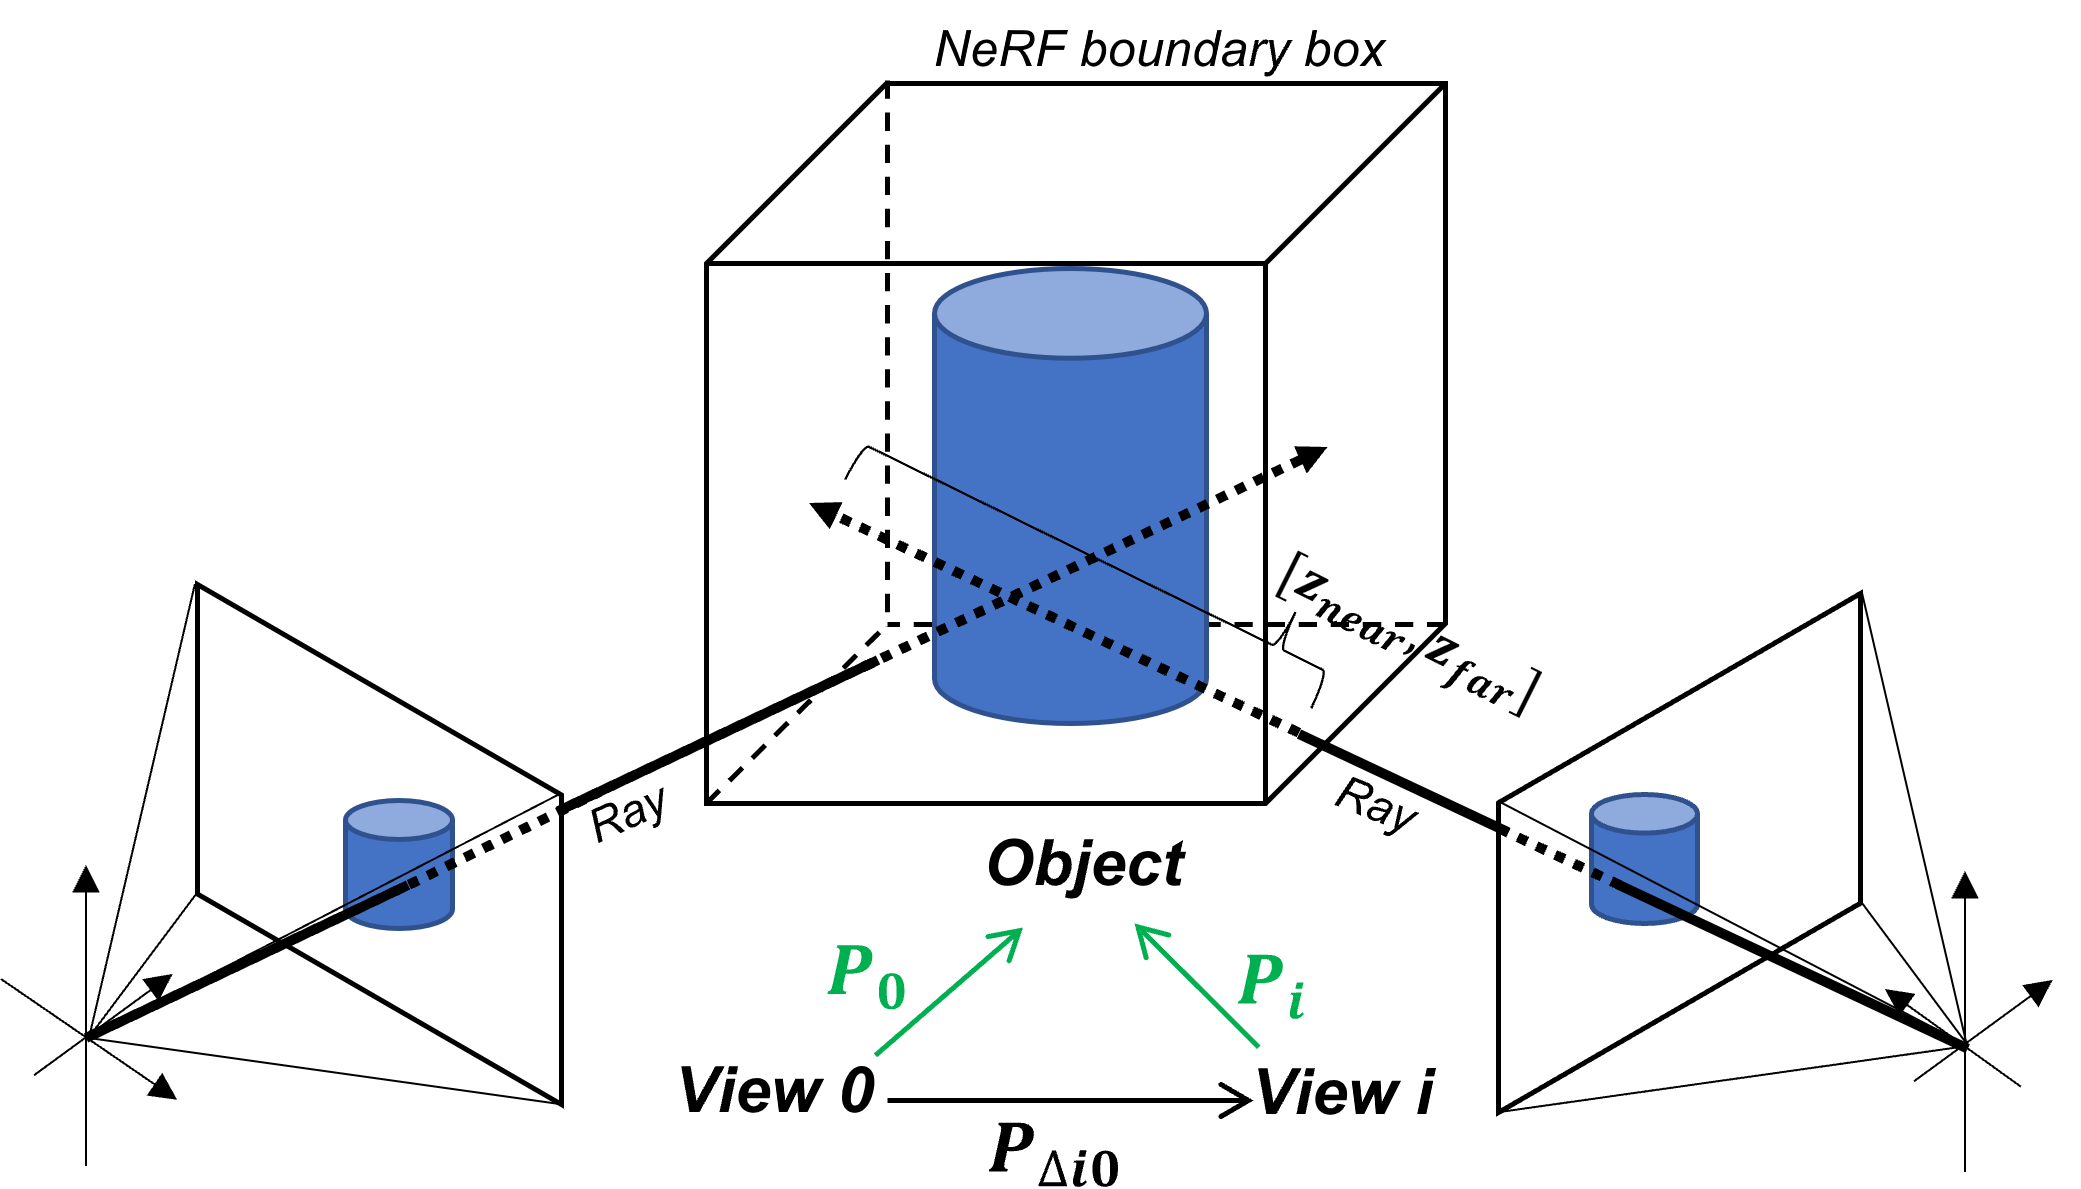}
        \caption{Weakly-supervised neural object reconstruction, in our problem setting.   
        }
    \label{fig:obj-nerf-m}
    \vspace{-0.5cm}
\end{figure}

\subsection{OBJ-NeRF}

Fig.~\ref{fig:obj-nerf-m} demonstrates the problem setting of our weakly-supervised object reconstruction. 
The object poses $\mathbf{P}_i$ in all frames are needed to construct the representation of the object. However, they are not provided in our settings. Instead, only relative camera poses $\mathbf{P}_{\Delta}$ are known. 
Based on the multi-view reconstruction theory, the scene can be reconstructed with respect to some reference coordinate systems using relative camera poses and RGB images. Additionally, 2D segmentation provides information about the object surface projection in 2D image which can help reconstruct the objects and separate them from the scene backgrounds.
Besides the shape, the object scale can also be estimated concurrently, because $\mathbf{P}_{\Delta}$ contains the absolute translation of the frames and thus constrains the size of the object. 
As we discussed, the relative pose and 2D segmentation are necessary to reconstruct the object. 

\begin{figure}
    \setlength{\belowcaptionskip}{-1cm}
    \centering
    \includegraphics[width=7cm]{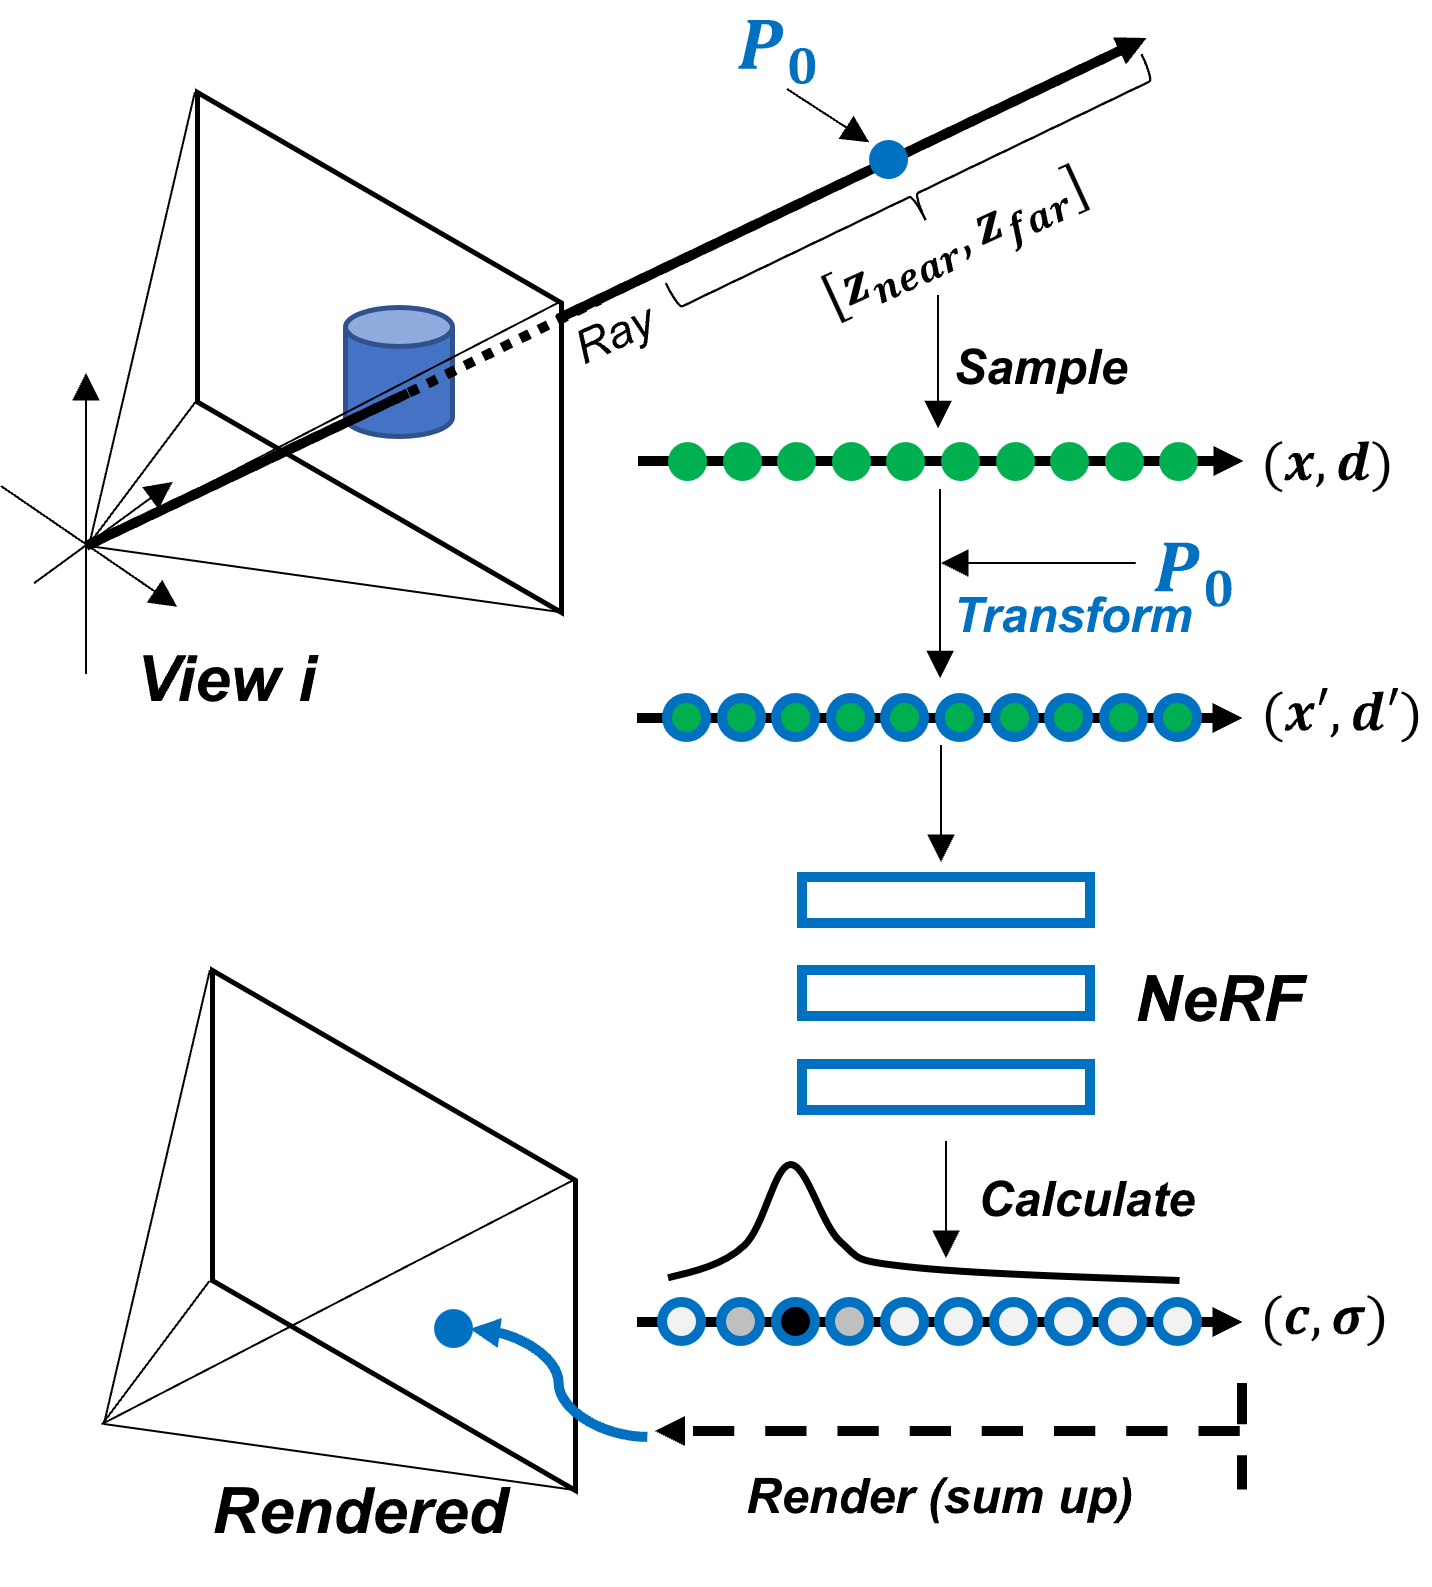}
        \caption{The OBJ-NeRF pipeline. First, a ray is generated from one pixel in image. 
        With estimated object pose $\mathbf{P}_0$, we can sample the discrete $N$ points according to the object center $t^{3d}$. 
        Then, we transform the sampled points from camera coordinate system to object-centric coordinate system by $\mathbf{P}_0$. \textit{This step newly defines the NeRF model canonical pose.} 
        The NeRF network encodes the object shape implicitly, which regresses the color and volume density of querying points. 
        With the regressed color and volume density of all points along the ray, the rendering operation can be applied to obtain the rendered pixel RGB value.
        }
    \label{fig:nerf-pipeline}
    \vspace{-0.5cm}
\end{figure}

OBJ-NeRF is built on top of NeRF network, and the differences between our OBJ-NeRF and original NeRF are: 
\begin{itemize}
    \item \textbf{Coordinate system.} The original NeRF is a scene-based reconstruction that refers to one camera frame. Instead, our OBJ-NeRF is an object-based reconstruction and defines the object canonical pose by optimizing object pose with respect to the reference frame.
    \item \textbf{Network Parameters.} Due to missing object pose in camera coordinate system which is needed in \textit{Rendering}, the object pose in the reference frame is optimized as the network parameters while training OBJ-NeRF.
    \item \textbf{Loss.} 2D segmentation is used to supervise the OBJ-NeRF network focusing on the object and ignoring the scene background. 
    \item \textbf{NOCS-map Render.} Apart from rendering the object mask and RGB image, the OBJ-NeRF network is extended to render NOCS-map, which can be used to supervise the training of the pose regression network. And,
    with the NOCS-map, the correspondences between the image pixel(2D) and Object(3D) can be built to estimate the object pose.
\end{itemize}

To make the description of OBJ-NeRF procedure more clear, We present the detailed OBJ-NeRF pipeline in Fig.~\ref{fig:nerf-pipeline}. 
\begin{figure}
    \setlength{\belowcaptionskip}{-1cm}
    \centering
    \includegraphics[width=6cm]{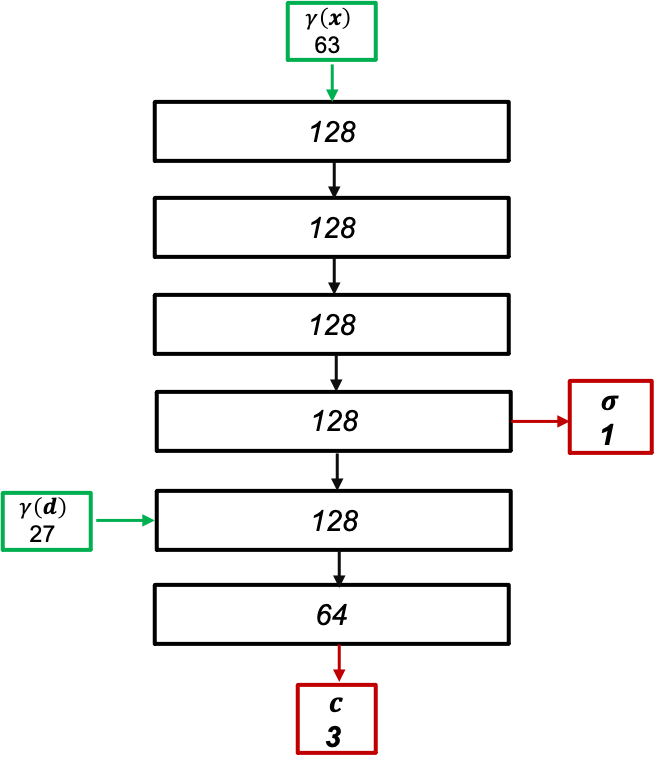}
        \caption{The network architecture of OBJ-NeRF. 
        }
    \label{fig:nerf-net}
    \vspace{-0.5cm}
\end{figure}
Following the network structure of original NeRF\cite{mildenhall2020nerf}, we use more lightweight MLPs. 
Original NeRF uses a total of 10 hidden layers where each of the first 9 hidden layers outputs a 256-dimensional feature vector and the last hidden layer outputs a 128-dimensional feature vector. 
In contrast, As shown in Fig.~\ref{fig:nerf-net}, we use a smaller MLP with only 4 hidden layers and each hidden layer outputs a 128-dimensional feature vector. Due to the low depth of our network, a skip connection as in the original NeRF architecture are not required. 
The positional encoding is firstly applied to the input 3-channel coordinate $\mathbf{x}$ and direction $\mathbf{d}$. Then the first four hidden layers take the input positional encoded coordinate as input and output the feature vector and the one channel volume density $\sigma$. The feature vector is be combined with the positional encoded direction and passed through the final hidden layers. Finally, the OBJ-NeRF outputs the 3-channel RGB value on this coordinate and direction.

\subsection{Pose Regression Network}

Our pose regression network is built on the top of the Resnet34~\cite{he2016resnet} pretrained from imagenet\cite{krizhevsky2012imagenet}. 
To obtain the high resolution regressed results, we mute the \textit{Maxpooing} layer before \textit{Block0} in Resnet34. Four upsampling layers are used to decode the features from the backbone network. And we add multi-head layers to separately predict the 1-channel mask and 3-channel \textit{NOCS}-map.

\begin{figure}
   \centering
    \includegraphics[width=7.5cm]{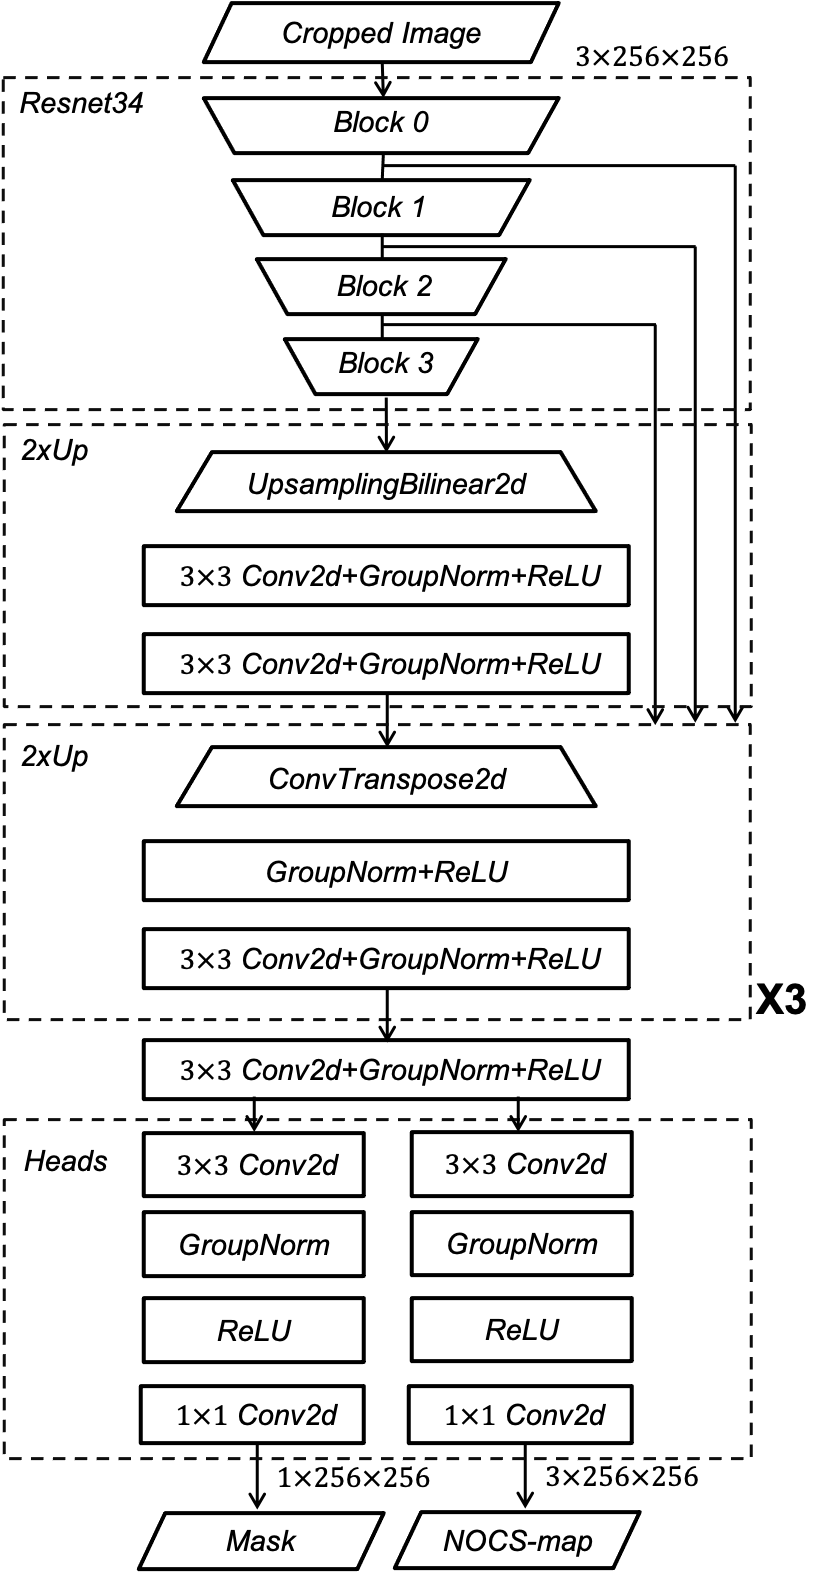}
        \caption{The network architecture of pose regression network. 
        }
    \label{fig:nerf-pipeline}
\end{figure}

We should again state that, the main focus of this paper is how to estimate the object pose with weak training labels available. So, we do not perform any model-based refinement methods. 

\section{NeRF-enabled PnP+RANSAC} \label{sec:ransac}
PnP+RANSAC algorithm is used to estimate the object pose from the 2D-3D correspondences. The basic idea is to select the best pose which has the most inliers. It can, however, be unstable if the number of correct correspondences is limited. 
% Benefit from the reconstructed object NeRF model.

Our goal is to find the object pose that ensures the high $Inlier Ratio$ Score and also keeps the high Intersection of Union between the regressed mask and the mask rendered with our trained NeRF. The detailed description of our proposed NeRF-enabled PnP+RANSAC algorithm is presented in Algorithm~\ref{alg:ransac}. The biggest difference from the original PnP+RANSAC method is the $Score$ used to select the best pose hypothesis. 
Based on $Inlier Ratio$, we add the mask-based $Precision$ and $Recall$ to make the whole algorithm more robust. The function $getInlierRatio$ calculate the inliers within the threshold $\tau$. As described in the paper, we convert the NeRF model into an octree structure to speed up the mask rendering to about 0.01s per image (about 1.5s by OBJ-NeRF). 

\section{Qualitative results} \label{sec:results}

We demonstrated additional qualitative results for LM~\cite{brachmann2014learning}, LM-O~\cite{brachmann2018learning} and HDB~\cite{kaskman2019homebreweddb} in Fig.~\ref{fig:lm-res-01} - \ref{fig:hbd-res-02}. 
We visualize the estimated 6D pose (blue) and its ground truth 6D poses (green) by overlaying the image with the corresponding transformed 3D bounding box. For better visualization we cropped the images and zoomed into the area of interest.
Moreover, we also visualize the NOCS-map ground truth rendered from the out well-trained OBJ-NeRF network, and the regressed NOCS-map from our pose regression network.

\begin{algorithm}[H]
\small
\SetAlgoLined
\KwResult{ $\hat{\mathbf{P}} \in SE(3)$  }
\KwIn{$ \hat{\mathbf{O}}, \hat{\mathbf{M}}, \mathcal{G}_{\psi}, K, N_{max}, \tau, p, v_1, v_2, v_3$}
$Score, iter \gets 0, 0$ \;
$N_{iter} \gets N_{max}$ \;
\While{ $iter > N_{max} ~or~ iter > N_{iter}$ } {
    Sample 5 samples $o$ from $\hat{\mathbf{O}}$ \;
    $\mathbf{P}_{est} \gets EPnP( o, K )$ \;
    $S_{ir} \gets getInlierRatio(\mathbf{P}_{est}, \hat{\mathbf{O}}, K, \tau)$ \;
    $\mathbf{M}_{nerf} \gets octreeNeRFRender(\mathcal{G}_{\psi}, \mathbf{P}_{est}, K)$\;
    $S_{Recall} \gets |\hat{\textbf{M}}_{nerf} \bigcap \hat{\textbf{M}}| / | \hat{\textbf{M}}| $ \;
    $S_{Prec} \gets |\hat{\textbf{M}}_{nerf} \bigcap \hat{\textbf{M}}| / |\hat{\textbf{M}} \bigcup  \hat{\textbf{M}}_{nerf}| $ \;
    $S \gets v_1 S_{IR} + v_2 S_{Recall} + v_3 S_{Prec}$ \;
    \If{ $S > Score $ }{
        $Socre \gets S$ \;
        $\hat{\mathbf{P}} \gets \mathbf{P}_{est}$ \;
     }
     $N_{iter} \gets log(1 - p) / log( 1 - ( 1 - Score)^5)$ \;
     $iter \gets iter + 1$ \;
}
\caption{NeRF-enabled PnP+RANSAC}
\label{alg:ransac}
\end{algorithm}

\begin{figure*}
   \centering
    \includegraphics[width=16cm]{figure/lm-res-01.png}
        \caption{Qualitative Results on LM~\cite{brachmann2014learning}. Columns (a) and (d) illustrate the visualization of our pose results(blue) and pose ground truth(green). Columns (b) and (e) are the rendered NOCS ground truth in the ground truth pose. Columns (c) and (f) are the regressed NOCS-map from our regression network.
        }
    \label{fig:lm-res-01}
\end{figure*}

\begin{figure*}
   \centering
    \includegraphics[width=16cm]{figure/lm-res-02.png}
        \caption{Qualitative Results on LM~\cite{brachmann2014learning}. Columns (a) and (d) illustrate the visualization of our pose results(blue) and pose ground truth(green). Columns (b) and (e) are the rendered NOCS ground truth in the ground truth pose. Columns (c) and (f) are the regressed NOCS-map from our regression network.
        }
    \label{fig:lm-res-02}
\end{figure*}

\begin{figure*}
   \centering
    \includegraphics[width=16cm]{figure/lmo-res-01.png}
        \caption{Qualitative Results on LM-O~\cite{brachmann2018learning}. Columns (a) and (d) illustrate the visualization of our pose results(blue) and pose ground truth(green). Columns (b) and (e) are the rendered NOCS ground truth in the ground truth pose. Columns (c) and (f) are the regressed NOCS-map from our regression network. 
        }
    \label{fig:lmo-res-01}
\end{figure*}

\begin{figure*}
   \centering
    \includegraphics[width=16cm]{figure/hbd-res-01.png}
        \caption{Qualitative Results on HBD~\cite{kaskman2019homebreweddb}. Columns (a) and (d) illustrate the visualization of our pose results(blue) and pose ground truth(green). Columns (b) and (e) are the rendered NOCS ground truth in the ground truth pose. Columns (c) and (f) are the regressed NOCS-map from our regression network.
        }
    \label{fig:hbd-res-01}
\end{figure*}

\begin{figure*}
   \centering
    \includegraphics[width=16cm]{figure/hbd-res-02.png}
        \caption{Qualitative Results on HBD~\cite{kaskman2019homebreweddb}. Columns (a) and (d) illustrate the visualization of our pose results(blue) and pose ground truth(green). Columns (b) and (e) are the rendered NOCS ground truth in the ground truth pose. Columns (c) and (f) are the regressed NOCS-map from our regression network.
        }
    \label{fig:hbd-res-02}
\end{figure*}
